# Supplementary material for: Kinematic Properties of Globally-Propagating Waves in the Solar Corona
Source: arXiv:1202.4360 source file (2012-02-20)
Supplement: Supplementary file 1 [file appendix.tex]

% this file is called up by thesis.tex
% content in this file will be fed into the main document
%\appendix
\chapter{Bibliography} % top level followed by section, subsection
\label{chap:bib}

% ----------------------- paths to graphics ------------------------

% change according to folder and file names
\ifpdf
    \graphicspath{{9_backmatter/figures/PNG/}{9_backmatter/figures/PDF/}{9_backmatter/figures/}}
\else
    \graphicspath{{9_backmatter/figures/EPS/}{9_backmatter/figures/}}
\fi

% ----------------------- contents from here ------------------------

\noindent 
\\ {\it 
Quote goes here
\begin{flushright}
Quoter goes here \\
\end{flushright}
 }

%General outline/introduction to be placed here
\vspace{15mm}

\section{Additional CBF identification plots}
\label{sect:app_app}

%\begin{figure*}
%\centerline{
%   \includegraphics[width=0.45\textwidth,clip=,trim=0mm 6mm 55mm 93mm]{space_broadening_b_20090213.eps}
%}
%\centerline{
%   \includegraphics[width=0.45\textwidth,clip=,trim=0mm 6mm 55mm 98mm]{time_broadening_b_20090213.eps}
%               }
%\caption{Similar to Figure~\ref{fig:broadening}, now only showing \emph{STEREO}-B data for the event on 2009~Feb~13.}
%\label{fig:app_broadening_20090213}
%\end{figure*}
